# Supplementary material for: Overcoming the Memory Bottleneck in Auxiliary Field Quantum Monte Carlo Simulations with Interpolative Separable Density Fitting
Source: arXiv:1810.00284 ancillary file (2018-12-21)
Supplement: Supplementary file 1 [file supplement.pdf]

# Supporting information for: 'Overcoming the Memory Bottleneck in Auxiliary Field Quantum Monte Carlo Simulations with Interpolative Separable Density Fitting'

Fionn D. Malone,* Shuai Zhang, and Miguel A. Morales*

*Quantum Simulations Group, Lawrence Livermore National Laboratory, 7000 East Avenue, Livermore, CA, 94551 USA.*

E-mail: malone14@llnl.gov; moralessilva2@llnl.gov

November 19, 2018

## Cohesive Energy

### Solid State calculation

To give some idea of the systematic errors remaining due to basis set and system size effects, in Fig. S1 we plot the AFQMC correlation energy of diamond in the DZVP and TZVP basis sets for the $2 \times 2 \times 2$, $3 \times 3 \times 3$ and $4 \times 4 \times 4$ supercells at the $T = 0$ K lattice constant. Note that the cohesive energy in the main text was computed at the $T = 300$ K lattice constant for comparison purposes. The extrapolated values are found to be -0.298 and -0.316 Ha/Cell respectively. The TZVP value for the $T = 300$ K lattice constant was found to be -0.311(7) Ha/Cell.

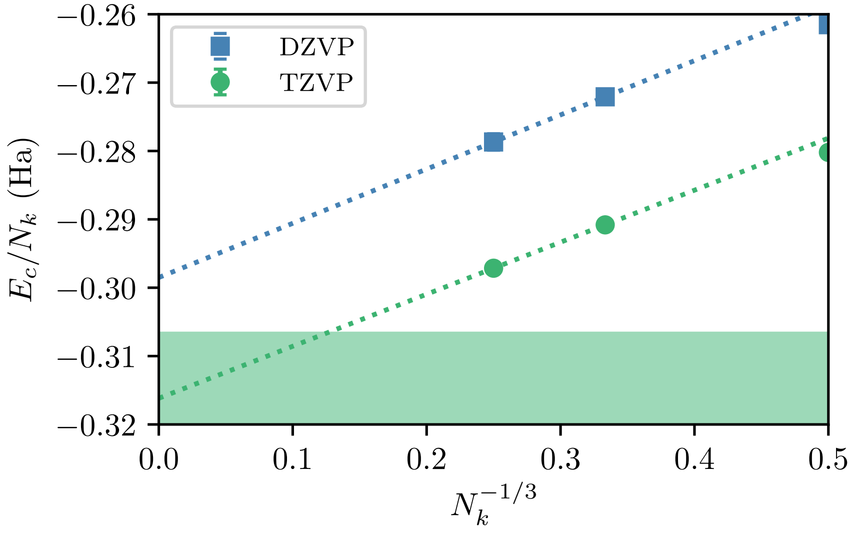


Figure S1: System size extrapolation of the correlation energy $E_c = E_{\mathrm{AFQMC}}(N_k) - E_{\mathrm{HF}}(N_k)$ with respect to the number of $k$-points, $N_k$. The shaded region gives a (conservative) estimate of the error bar from $\frac{1}{2}|E_c(N_k = \infty) - E_c(N_k = 64)|$.

.

## Atomic calculation

In Fig. S2 we present the basis set extrapolation performed to compute the atomic energy of carbon. To compute the atomic energy we set 'cell.dimension == 0' in PySCF[S1] and performed a UHF calculation for the triplet spin state ('cell.spin = 2') of a single carbon atom.

# Population Control

In Fig. S3 we plot the dependence of the total energy on walker population for a $3 \times 3 \times 3$ supercell of diamond in the TZVP basis set at $a = 3.57$ Å. Any population control bias is seen to be essentially negligible (all points are within error bars), which is likely as a result of diamond being well described by RHF and thus the constraint is fairly weak.

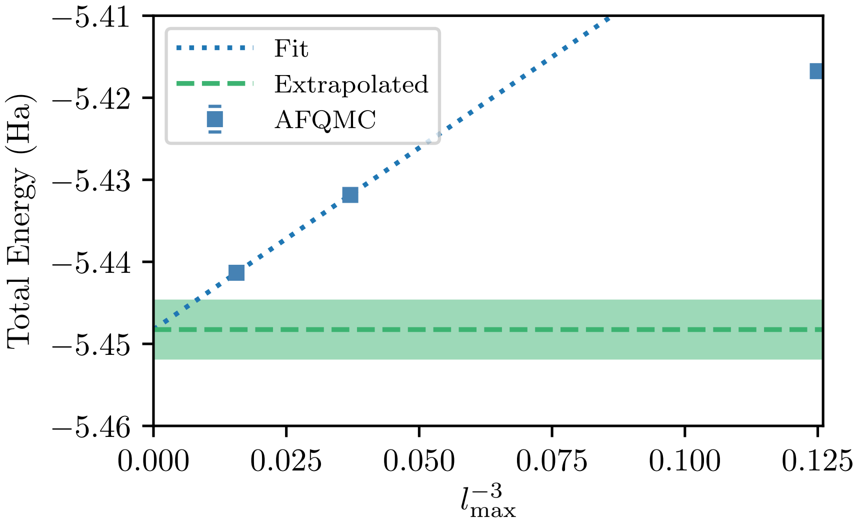


Figure S2: Basis set extrapolation of the atomic energy of Carbon assuming an $l_{\text{max}}^{-3}$ dependence on the total energy, where $l_{\text{max}}$ is the maximum angular momentum contained in the basis set. The final error bar (shown as the dashed green region) is estimated as $\frac{1}{2}(E(\text{CBS}) - E(\text{GTH-CC-PVQZ}))$

.

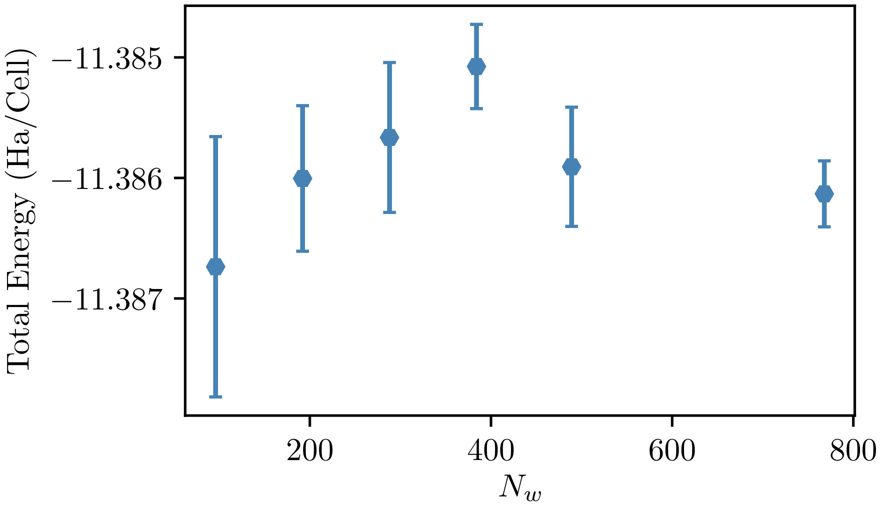


Figure S3: Dependence of total energy $3 \times 3 \times 3$ supercell of diamond in the TZVP basis set at $a = 3.57$ Å.

.

## References

(S1) Sun, Q.; Berkelbach, T. C.; Blunt, N. S.; Booth, G. H.; Guo, S.; Li, Z.; Liu, J.; McClain, J. D.; Sayfutyarova, E. R.; Sharma, S.; Wouters, S.; Chan, G. K. L. PySCF: the Python-based simulations of chemistry framework. *WIREs Comput. Mol. Sci.* **2017**, *8*, e1340.
